# Supplementary material for: GNN's Uncertainty Quantification using Self-Distillation
Source: arXiv:2506.20046 source file (2025-06-24)
Supplement: Supplementary file 1 [file appendices.tex]

\section{Appendix}\label{sec:appendix}
